# Supplementary material for: Challenging Language-Dependent Segmentation for Arabic: An Application to Machine Translation and Part-of-Speech Tagging
Source: arXiv:1709.00616 source file (2017-09-02)
Supplement: Supplementary file 1 [file appendix.tex]

\section{Appendix}

The Figures \ref{fig.ngram_farasa},\ref{fig.ngram_cnn}, \ref{fig.ngram_bpe10k}, and \ref{fig.ngram_word} shows the various errors result of the experimentation using {\tt MORPH}, {\tt CHAR}, {\tt BPE}, and {\tt UNSEG} respectively. JUS was the common error between all the system because its presence in the corpus is very low and therefore it is hard to model. Given the example ``\<فلنقل>'' ``flnql'' (so to say) which is suppose to be analyzed as {\tt CONJ JUS V} it gets analyzed as {\tt CONJ PREP NOUN} as if it meant (so for moving). Most of the times this former example appears in the start of a sentence and therefore not much context can assist in such instance. Another common error is the cases for ADJ that gets analyzed as NUM or NOUN. An example is the case of ``\<المنبر>'' ``Almnbr'' (the pulit) that was analyzed in some instances as {\tt DET ADJ} instead of {\tt DET NOUN}. Handling the numbers also is very challenging. The numbers spelled in digits are hard to capture without extra processing as they do not occur frequently enough. ``\<٧.٥٦٧ بليون>'' ``70567 blywn'' (70567 billion) as an example which was predicted as {\tt NOUN NOUN} while the proper analysis should be {\tt NUM NOUN}

\begin{figure}[h]
\includegraphics[width=\linewidth]{Rplot0_ngram_farasa.pdf}
\caption{Confusion matrix for {\tt MORPH} showing prediction errors for labels such as FOREIGN, JUS, and ADJ which were classified as other tags. }
\label{fig.ngram_farasa}
\end{figure}

\begin{figure}[h]
\includegraphics[width=\linewidth]{Rplot0_ngram_cnn.pdf}
\caption{Confusion matrix for {\tt CHAR} showing prediction errors for labels such as FOREIGN, JUS,FUT\_PART, ADV and ADJ which were classified as other tags. }
\label{fig.ngram_cnn}
\end{figure}

\begin{figure}[h]
\includegraphics[width=\linewidth]{Rplot0_ngram_bpe10k.pdf}
\caption{Confusion matrix for {\tt BPE} showing prediction errors for labels such as FOREIGN, JUS, and ADJ which were classified as other tags. }
\label{fig.ngram_bpe10k}
\end{figure}

\begin{figure}[h]
\includegraphics[width=\linewidth]{Rplot0_ngram_word.pdf}
\caption{Confusion matrix for {\tt UNSEG} showing prediction errors for labels such as FOREIGN, JUS, and ADJ which were classified as other tags. }
\label{fig.ngram_word}
\end{figure}
